# Supplementary material for: Estimating Extreme 3D Image Rotation with Transformer Cross-Attention
Source: arXiv:2303.02615 source file (2024-03-08)
Supplement: Supplementary file 1 [file final_main_table_supp.tex]

\definecolor{graytext}{RGB}{130,130,130}

\begin{table*}[t]
\setlength{\tabcolsep}{1.0pt}

 \footnotesize
\scriptsize
\begin{center}
\begin{tabularx}{\textwidth}{llccclccclccclccclccc}
\toprule
\multicolumn{2}{l}{}& \multicolumn{3}{c}{InteriorNet} &  & \multicolumn{3}{c}{InteriorNet-T} &  & \multicolumn{3}{c}{SUN360} &  & \multicolumn{3}{c}{StreetLearn} &  & \multicolumn{3}{c}{StreetLearn-T}\\ \cline{3-5} \cline{7-9} \cline{11-13} \cline{15-17} \cline{19-21}
Overlap 
& Method
& Avg(\degree$\downarrow$) & Med(\degree$\downarrow$) & \multicolumn{1}{c}{10\degree(\%$\uparrow$)} & & Avg(\degree$\downarrow$) & Med(\degree$\downarrow$) & \multicolumn{1}{c}{10\degree(\%$\uparrow$)} &  & Avg(\degree$\downarrow$) & Med(\degree$\downarrow$) & \multicolumn{1}{c}{10\degree(\%$\uparrow$)} &  & Avg(\degree$\downarrow$) & Med(\degree$\downarrow$) & \multicolumn{1}{c}{10\degree(\%$\uparrow$)} &  & Avg(\degree$\downarrow$) & Med(\degree$\downarrow$) & \multicolumn{1}{c}{10\degree(\%$\uparrow$)} \\ \midrule
\multirow{13}{*}{Large} %&  SIFT*~\cite{lowe2004distinctive}       & 6.09                 & 4.00                 & 84.86               &  & 7.78                 & 2.95                 & 55.52               &  & 5.46                       & 3.88                       & 93.10                      &  & 5.84                 & 3.16                 & 91.18               &  & 18.86                & 3.13                 & 22.37               \\
                         & SIFT*~\cite{lowe2004distinctive}       & 6.09                 & 4.00                 & 84.86               &  & 7.78                 & 2.95                 & 55.52               &  & 5.46                       & 3.88                       & 93.10                      &  & 5.84                 & 3.16                 & 91.18               &  & \color{graytext}{18.86}                & \color{graytext}{3.13}                 & \color{graytext}{22.37}               \\
                         & D2-Net*~\cite{Dusmanu2019CVPR}         & 8.27                 & 3.78                 & 69.48               &  & \color{graytext}{14.19}                & \color{graytext}{9.38}                 & \color{graytext}{15.82}               &  & 10.48                      & 4.22                       & 69.46                      &  & 12.85                & 4.42                 & 54.12               &  & \color{graytext}{8.76}                 & \color{graytext}{6.73}                 & \color{graytext}{1.32}                \\
                         %& SuperPoint*~\cite{detone18superpoint}  & 5.40                 & 3.53                 & 87.10               &  & 5.46                 & 2.79                 & 65.97               &  & 4.69                       & 3.18                       & 92.12                      &  & 6.23                 & 3.61                 & 91.18               &  & \textbf{6.38}        & \textbf{1.79}        & 16.45               \\
                         & SuperPoint*~\cite{detone18superpoint}  & 5.40                 & 3.53                 & 87.10               &  & 5.46                 & 2.79                 & 65.97               &  & 4.69                       & 3.18                       & 92.12                      &  & 6.23                 & 3.61                 & 91.18               &  & \color{graytext}{6.38}        & \color{graytext}{1.79}        & \color{graytext}{16.45}               \\
                         & RegEuler-o                            & 4.89                 & 3.52                 & 91.56               &  & 8.36                 & 4.64                 & 80.00               &  & 6.57                       & 5.16                       & 85.22                      &  & 3.99                 & 3.20                 & 95.29               &  & 15.15                & 7.13                 & 62.50               \\
                         & RegEuler                               & 11.11                & 7.92                 & 60.05               &  & 20.98                & 14.59                & 33.43               &  & 14.19          & 10.77         & 46.31                       &  & 27.47                & 17.59                & 23.53               &  & 46.89                & 32.36                & 11.84               \\
                         & Reg4D~\cite{en2018rpnet}-o            & 4.95                 & 3.47                 & 91.56               &  & 9.58                 & 7.00                 & 69.25               &  & 7.86                       & 5.89                       & 76.85                      &  & 3.14                 & 2.67                 & 98.82               &  & 11.73                & 6.35                 & 74.34               \\
                         & Reg4D~\cite{en2018rpnet}            & 13.83                & 10.26                & 48.88               &  & 26.05                & 16.84                & 22.99               &  & 36.02                      & 24.23                      & 16.26                      &  & 20.57                & 13.05                & 40.00               &  & 41.44                & 28.27                & 20.39               \\
                         & Reg6D~\cite{zhou2019continuity}-o-128 & 7.48                 & 5.24                 & 75.19               &  & 14.58                & 10.97                & 46.27               &  & 11.97                      & 8.11                       & 57.64                      &  & 6.00                 & 5.20                 & 85.29               &  & 13.66                & 8.24                 & 58.55               \\
                         & Reg6D~\cite{zhou2019continuity}-128    & 14.04                & 9.06                 & 53.10               &  & 31.96                & 21.19                & 22.99               &  & 40.19                      & 33.41                      & 8.87                       &  & 14.09                & 8.63                 & 56.47               &  & 31.01                & 19.14                & 26.97               \\
                         & Reg6D~\cite{zhou2019continuity}-o     & 5.43                 & 3.87                 & 87.10               &  & 10.45                & 6.91                 & 67.76               &  & 7.18                       & 5.79                       & 81.28                      &  & 3.36                 & 2.71                 & 97.65               &  & 12.31                & 6.02                 & 69.08               \\
                         & Reg6D~\cite{zhou2019continuity}        & 9.05                 & 5.90                 & 68.49               &  & 17.00                & 11.95                & 41.79               &  & 16.51                      & 12.43                      & 40.39                      &  & 11.70                & 8.87                 & 58.24               &  & 36.71                & 24.79                & 23.03               \\
                         & Ours-o                                & \textbf{1.53}        & 1.10                 & \textbf{99.26}     &  & \textbf{2.89}        & \textbf{1.10}        & \textbf{97.61}     &  & \textbf{1.00}              & \textbf{0.94}              & \textbf{100.00}           &  & \textbf{1.19}        & \textbf{1.02}        & \textbf{99.41}     &  & 9.12                 & 2.91                 & \textbf{87.50}     \\
                         & Ours                                   & 1.82                 & \textbf{0.88}        & 98.76               &  & 8.86                 & 1.86                 & 93.13               &  & 1.37                       & 1.09                       & 99.51                      &  & 1.52                 & 1.09                 & \textbf{99.41}     &  & 24.98                & 2.48                 & 78.95               \\
\midrule %\cline{2-21}
                        % & Training                               & 0.77          & 0.71          & 99.73          &  & 2.15           & 1.36          & 98.71          &  & 0.81          & 0.80          & 100.00          &  & 1.03          & 0.92          & 99.96          &  & 3.49          & 1.28          & 96.91          \\ \midrule
\multirow{13}{*}{Small} %& SIFT*~\cite{lowe2004distinctive}       & 24.18                & 8.57                 & 39.73               &  & 18.16                & 10.01                & 18.52               &  & 13.71                      & 6.33                       & 56.77                      &  & 16.22                & 7.35                 & 55.81               &  & 38.78                & 13.81                & 5.68                \\
                         & SIFT*~\cite{lowe2004distinctive}       & 24.18                & 8.57                 & 39.73               &  & \color{graytext}{18.16}                & \color{graytext}{10.01}                & \color{graytext}{18.52}               &  & 13.71                      & 6.33                       & 56.77                      &  & 16.22                & 7.35                 & 55.81               &  & \color{graytext}{38.78}                & \color{graytext}{13.81}                & \color{graytext}{5.68}                \\
                         & D2-Net*~\cite{Dusmanu2019CVPR}         & \color{graytext}{14.21}                & \color{graytext}{8.50}                 & \color{graytext}{3.42}                &  & \color{graytext}{--}                   & \color{graytext}{--}                   & \color{graytext}{0.00}                &  & \color{graytext}{25.49}                      & \color{graytext}{9.17}                       & \color{graytext}{4.51}                       &  & \color{graytext}{41.35}                & \color{graytext}{18.43}                & \color{graytext}{1.66}                &  & \color{graytext}{67.27}                & \color{graytext}{67.27}                & \color{graytext}{0.00}                \\
                         %& SuperPoint*~\cite{detone18superpoint}  & 16.72                & 8.43                 & 21.58               &  & 11.61                & 5.82                 & 11.73               &  & 17.63                      & 7.70                       & 26.69                      &  & 19.29                & 7.60                 & 24.58               &  & \textbf{6.80}        & 6.85                 & 0.95                \\
                         & SuperPoint*~\cite{detone18superpoint}  & \color{graytext}{16.72}                & \color{graytext}{8.43}                 & \color{graytext}{21.58}               &  & \color{graytext}{11.61}                & \color{graytext}{5.82}                 & \color{graytext}{11.73}               &  & \color{graytext}{17.63}                      & \color{graytext}{7.70}                       & \color{graytext}{26.69}                      &  & \color{graytext}{19.29}                & \color{graytext}{7.60}                 & \color{graytext}{24.58}               &  & \color{graytext}{6.80}        & \color{graytext}{6.85}                 & \color{graytext}{0.95}                \\
                         & RegEuler-o                            & 15.37                & 7.88                 & 59.59               &  & 19.27                & 7.41                 & 64.51               &  & 14.88                      & 8.92                       & 54.14                      &  & 8.24                 & 4.29                 & 86.71               &  & 20.41                & 9.96                 & 50.47               \\
                         & RegEuler                               & 28.58                & 17.77                & 31.85               &  & 32.87                & 21.96                & 18.52               &  & 32.28          & 25.41         & 12.41                       &  & 52.08                & 37.35                & 4.32                &  & 58.43                & 47.27                & 7.57                \\
                         & Reg4D~\cite{en2018rpnet}-o            & 16.62                & 8.46                 & 57.88               &  & 24.77                & 12.42                & 41.67               &  & 15.02                      & 9.81                       & 51.88                      &  & 6.55                 & 4.15                 & 91.03               &  & 14.56                & 7.46                 & 65.93               \\
                         & Reg4D~\cite{en2018rpnet}            & 32.86                & 22.41                & 15.75               &  & 41.52                & 28.46                & 10.80               &  & 66.59                      & 57.84                      & 0.38                       &  & 38.39                & 24.77                & 10.63               &  & 50.42                & 34.07                & 15.46               \\
                         & Reg6D~\cite{zhou2019continuity}-o-128 & 22.45                & 12.57                & 38.70               &  & 31.15                & 16.58                & 27.47               &  & 23.17                      & 15.08                      & 24.06                      &  & 9.12                 & 5.71                 & 82.06               &  & 20.70                & 10.69                & 45.43               \\
                         & Reg6D~\cite{zhou2019continuity}-128    & 36.37                & 23.81                & 18.84               &  & 54.24                & 39.94                & 14.81               &  & 67.97                      & 60.91                      & 0.38                       &  & 24.03                & 15.13                & 30.56               &  & 41.07                & 28.33                & 17.03               \\
                         & Reg6D~\cite{zhou2019continuity}-o     & 17.83                & 9.61                 & 51.37               &  & 21.87                & 11.43                & 44.14               &  & 18.61                      & 11.66                      & 39.85                      &  & 7.95                 & 4.34                 & 87.71               &  & 15.07                & 7.59                 & 63.41               \\
                         & Reg6D~\cite{zhou2019continuity}        & 25.71                & 15.56                & 33.56               &  & 42.93                & 28.92                & 23.15               &  & 42.55                      & 32.11                      & 9.40                       &  & 24.77                & 15.11                & 30.56               &  & 46.61                & 34.33                & 13.88               \\
                         & Ours-o                                & 6.45                 & 1.61                 & 95.89               &  & \textbf{10.24}       & \textbf{1.38}        & \textbf{89.81}     &  & \textbf{3.09}              & \textbf{1.41}              & \textbf{98.50}            &  & \textbf{2.32}        & \textbf{1.41}        & \textbf{98.67}     &  & \textbf{13.04}                & 3.49                 & \textbf{84.23}     \\
                         %& Ours                                   & \textbf{4.31}        & \textbf{1.16}        & \textbf{96.58}     &  & 30.43                & 2.63                 & 74.07               &  & 6.13                       & 1.77                       & 95.86                      &  & 3.23                 & \textbf{1.41}        & 98.34               &  & 27.84                & \textbf{3.19}        & 74.76               \\
                         & Ours                                   & \textbf{4.31}        & \textbf{1.16}        & \textbf{96.58}     &  & 30.43                & 2.63                 & 74.07               &  & 6.13                       & 1.77                       & 95.86                      &  & 3.23                 & \textbf{1.41}        & 98.34               &  & 27.84                & \textbf{3.19}        & 74.76               \\
 \midrule %\cline{2-21}
                        % & Training                               & 3.57          & 0.88          & 98.34          &  & 9.13           & 1.47          & 94.75          &  & 1.81          & 1.03          & 99.26           &  & 1.46          & 1.13          & 99.80          &  & 4.23          & 1.44          & 96.22          \\ \midrule
\multirow{8}{*}{None}   %& SIFT*~\cite{lowe2004distinctive}       & 109.30               & 92.86                & 0.00                &  & 93.79                & 113.86               & 0.00                &  & 127.61                     & 129.07                     & 0.00                       &  & 83.49                & 90.00                & 0.38                &  & 85.90                & 106.84               & 0.38                \\
                         & SIFT*~\cite{lowe2004distinctive}       & \color{graytext}{109.30}               & \color{graytext}{92.86}                & \color{graytext}{0.00}                &  & \color{graytext}{93.79}                & \color{graytext}{113.86}               & \color{graytext}{0.00}                &  & \color{graytext}{127.61}                     & \color{graytext}{129.07}                     & \color{graytext}{0.00}                       &  & \color{graytext}{83.49}                & \color{graytext}{90.00}                & \color{graytext}{0.38}                &  & \color{graytext}{85.90}                & \color{graytext}{106.84}               & \color{graytext}{0.38}                \\
                         & D2-Net*~\cite{Dusmanu2019CVPR}         & \color{graytext}{--}                   & \color{graytext}{--}                   & \color{graytext}{0.00}                &  & \color{graytext}{--}                   & \color{graytext}{--}                   & \color{graytext}{0.00}                &  & \color{graytext}{171.21}                     & \color{graytext}{171.21}                     & \color{graytext}{0.00}                       &  & \color{graytext}{--}                   & \color{graytext}{--}                   & \color{graytext}{0.00}                &  & \color{graytext}{--}                   & \color{graytext}{--}                   & \color{graytext}{0.00}                \\
                         %& SuperPoint*~\cite{detone18superpoint}  & 120.28               & 120.28               & 0.00                &  & --                   & --                   & 0.00                &  & 149.80                     & 165.24                     & 0.00                       &  & --                   & --                   & 0.00                &  & --                   & --                   & 0.00                \\
                         & SuperPoint*~\cite{detone18superpoint}  & \color{graytext}{120.28}               & \color{graytext}{120.28}               & \color{graytext}{0.00}                &  & \color{graytext}{--}                   & \color{graytext}{--}                   & \color{graytext}{0.00}                &  & \color{graytext}{149.80}                     & \color{graytext}{165.24}                     & \color{graytext}{0.00}                       &  & \color{graytext}{--}                   & \color{graytext}{--}                   & \color{graytext}{0.00}                &  & \color{graytext}{--}                   & \color{graytext}{--}                   & \color{graytext}{0.00}                \\
                         & RegEuler                               & 52.95                & 36.03                & 7.87                &  & 55.73                & 42.04                & 9.97                & & 70.93          & 59.43         & 5.46                       &  & 55.92                & 41.23                & 7.56                &  & 61.04                & 48.79                & 9.04                \\
                         & Reg4D~\cite{en2018rpnet}            & 62.04                & 48.92                & 4.59                &  & 59.85                & 48.81                & 4.99                &  & 80.08                      & 72.78                      & 1.32                       &  & 46.19                & 32.74                & 9.26                &  & 55.70                & 39.70                & 9.79                \\
                         & Reg6D~\cite{zhou2019continuity}-128    & 64.59                & 49.80                & 5.90                &  & 79.86                & 71.60                & 5.87                &  & 83.29                      & 75.08                      & 0.56                       &  & 34.78                & 23.16                & 17.77               &  & 50.96                & 36.50                & 9.23                \\
                         & Reg6D~\cite{zhou2019continuity}        & 48.36                & 32.93                & 10.82               &  & 60.91                & 51.26                & 11.14               &  & 64.74                      & 56.55                      & 3.77                       &  & 28.48                & 18.86                & 24.39               &  & 49.23                & 35.66                & 11.86               \\
                         & Ours                                   & \textbf{37.69}       & \textbf{3.15}        & \textbf{61.97}     &  & \textbf{49.44}       & \textbf{4.17}        & \textbf{58.36}     &  & \textbf{34.92}             & \textbf{4.43}              & \textbf{61.39}            &  & \textbf{5.77}        & \textbf{1.53}        & \textbf{96.41}     &  & \textbf{30.98}       & \textbf{3.50}        & \textbf{72.69}     \\
\midrule% \cline{2-21}
                        % & Training                               & 26.16         & 1.41          & 73.21          &  & 19.71          & 2.04          & 84.97          &  & 27.18         & 2.02          & 69.51           &  & 3.18          & 1.36          & 98.62          &  & 18.41         & 1.94          & 83.50          \\ \midrule
\multirow{8}{*}{All}    %& SIFT*~\cite{lowe2004distinctive}       & 13.68                & 5.04                 & 45.80               &  & 12.24                & 5.69                 & 24.60               &  & 18.12                      & 5.02                       & 34.00                      &  & 17.29                & 5.53                 & 32.50               &  & 36.00                & 6.03                 & 5.40                \\
                         & SIFT*~\cite{lowe2004distinctive}       & 13.68                & 5.04                 & 45.80               &  & \color{graytext}{12.24}                & \color{graytext}{5.69}                 & \color{graytext}{24.60}               &  & \color{graytext}{18.12}                      & \color{graytext}{5.02}                       & \color{graytext}{34.00}                      &  & \color{graytext}{17.29}                & \color{graytext}{5.53}                 & \color{graytext}{32.50}               &  & \color{graytext}{36.00}                & \color{graytext}{6.03}                 & \color{graytext}{5.40}                \\
                         & D2-Net*~\cite{Dusmanu2019CVPR}         & \color{graytext}{8.56}                 & \color{graytext}{3.95}                 & \color{graytext}{29.00}               &  & \color{graytext}{14.19}                & \color{graytext}{9.38}                 & \color{graytext}{5.30}                &  & \color{graytext}{13.80}                      & \color{graytext}{4.62}                       & \color{graytext}{15.30}                      &  & \color{graytext}{16.41}                & \color{graytext}{5.38}                 & \color{graytext}{9.70}                &  & \color{graytext}{23.39}                & \color{graytext}{11.87}                & \color{graytext}{0.20}                \\
                         %& SuperPoint*~\cite{detone18superpoint}  & \textbf{8.19}        & 4.08                 & 41.40               &  & \textbf{6.62}        & 3.38                 & 25.90               &  & \textbf{11.09}             & 4.00                       & 25.80                      &  & 11.52                & 4.80                 & 22.90               &  & \textbf{6.42}        & \textbf{2.62}        & 2.80                \\
                         %& SuperPoint*~\cite{detone18superpoint}  & \textbf{8.19}        & 4.08                 & 41.40               &  & \textbf{6.62}        & 3.38                 & 25.90               &  & \textbf{11.09}             & 4.00                       & 25.80                      &  & 11.52                & 4.80                 & 22.90               &  & \color{graytext}{6.42}        & \color{graytext}{2.62}        & 2.80                \\
                         & SuperPoint*~\cite{detone18superpoint}  & \color{graytext}{8.19}        & \color{graytext}{4.08}                 & \color{graytext}{41.40}               &  & \color{graytext}{6.62}        & \color{graytext}{3.38}                 & \color{graytext}{25.90}               &  & \color{graytext}{11.09}             & \color{graytext}{4.00}                       & \color{graytext}{25.80}                      &  & \color{graytext}{11.52}                & \color{graytext}{4.80}                 & \color{graytext}{22.90}               &  & \color{graytext}{6.42}        & \color{graytext}{2.62}        & \color{graytext}{2.80}                \\
                         & RegEuler                               & 28.97                & 15.53                & 35.90               &  & 36.68                & 22.70                & 20.60               &  & 49.13          & 31.44         & 15.60                       &  & 49.93                & 35.08                & 9.30                &  & 58.06                & 45.54                & 9.00                \\
                         & Reg4D~\cite{en2018rpnet}          & 34.09                & 19.59                & 25.70               &  & 42.59                & 28.35                & 12.90               &  & 67.55                      & 55.40                      & 4.10                       &  & 39.48                & 25.76                & 14.90               &  & 51.86                & 36.89                & 13.20               \\
                         & Reg6D~\cite{zhou2019continuity}-128    & 35.98                & 18.65                & 28.70               &  & 55.51                & 36.90                & 14.50               &  & 70.46                      & 57.87                      & 2.20                       &  & 28.03                & 17.11                & 28.20               &  & 44.79                & 31.00                & 14.40               \\
                         & Reg6D~\cite{zhou2019continuity}        & 25.90                & 13.02                & 40.70               &  & 40.38                & 23.35                & 25.30               &  & 49.05                      & 34.37                      & 12.70                      &  & 24.51                & 15.31                & 32.00               &  & 46.50                & 33.14                & 29.90               \\
                         %& Ours                                   & 13.49                & \textbf{1.18}        & \textbf{86.90}     &  & 29.68                & \textbf{2.58}        & \textbf{75.10}     &  & 20.45                      & \textbf{2.23}              & \textbf{78.30}            &  & \textbf{4.40}        & \textbf{1.44}        & \textbf{97.50}     &  & 29.85                & 3.20                 & \textbf{74.30}     \\
                         & Ours                                   & \textbf{13.49}                & \textbf{1.18}        & \textbf{86.90}     &  & \textbf{29.68}                & \textbf{2.58}        & \textbf{75.10}     &  & \textbf{20.45}                      & \textbf{2.23}              & \textbf{78.30}            &  & \textbf{4.40}        & \textbf{1.44}        & \textbf{97.50}     &  & \textbf{29.85}                & \textbf{3.20}                 & \textbf{74.30}     \\ %\cline{2-21}
                        % & Training                               & 9.77          & 0.91          & 90.80          &  & 10.84          & 1.60          & 92.40          &  & 14.66         & 1.25          & 84.10           &  & 2.58          & 1.19          & 98.96          &  & 15.90         & 1.78          & 85.79         \\ 
                        \bottomrule 
\end{tabularx}
\end{center}
\vspace{-5pt}
\caption{\textbf{Rotation estimation evaluation on the InteriorNet, SUN360, and StreetLearn datasets.} 
We report the mean and median geodesic error in degrees, and the percentage of pairs with a relative rotation error under 10$\degree$, for different overlapping levels (Large, Small, and None), as detailed in Section 4.3 of the main paper. For the percentage of pairs (10$\degree$\%), higher is better. Models trained only on overlapping pairs are denoted with ``-o''.
% *Note that SIFT, D2-Net, and SuperPoint fail to output an estimated rotation matrix for some image pairs. We disregard these for the mean and median error computation.
*For the indicated methods, mean and median errors are computed only over successful image pairs, for which these algorithms output an estimated rotation matrix (cases where there is failure over more than $50\%$ of the test pairs is shown in gray). 
}
\label{tab:main_result_supp}
\end{table*}
